# Supplementary material for: Experimenting a New Programming Practice with LLMs
Source: arXiv:2401.01062 source file (2024-01-02)
Supplement: Supplementary file 1 [file appendix.tex]

\section{A}\label{appendixA}
